# Supplementary material for: Piecing Together Clues: A Benchmark for Evaluating the Detective Skills of Large Language Models
Source: arXiv:2307.05113 source file (2024-03-20)
Supplement: Supplementary file 1 [file 07.Appendix.01.tex]

\input{tables/tab_annotation}

\begin{table*}[t]
    \centering
    \resizebox{\textwidth}{!}{
    \begin{tabular}{|c|l|}
    \hline
        \textbf{Purpose} & \textbf{Prompt} \\
        \hline
        \multicolumn{2}{|l|}{\cellcolor{mygray}\textit{Detective Thinking}}
        \\
        \hline
        
        \multirow{3}{*}{Detail Detection} & 
        Read the following passage carefully and identify as many details as you can. Pay
        \\&
        attention to descriptions, actions, and characters. Use your observational skills to
        \\&
        identify anything else that might be of significance.
        \\
        \hline
        \multirow{4}{*}{Detail Connection} & 
        Using the details you have identified from the context, draw connections and analyze
        \\&
        the relationships between them. Consider the significance of each detail and how it
        \\&
        relates to the larger meaning of the text. Look for patterns, symbolism, and other
        \\&
        elements that may help explain why the author included these specific details.\\
        \hline
        \multirow{5}{*}{Answer Inspiration} & 
        Using the details you have identified and the
        \\&
        clues you have drawn from the given question, analyze their connections and draw
        \\&
        conclusions about the larger meaning of the text. Consider the significance of each
        \\&
        detail and how it relates to the question. Look for themes, motifs, and other
        \\&
        elements that may help explain why the author included these specific details and clues.\\
        \hline
        \multirow{4}{*}{Weighted Reasoning} & 
        Answer the question by taking the raw context into consideration but mainly using the 
        \\&
        conclusion and the details you have drawn before. Remember the connection between your
        \\&
        drawn details and the conclusion to the question, don't be disturbed by the irrelevant
        \\&
        information in the context.
        \\
        \hline
        \multicolumn{2}{|l|}{\cellcolor{mygray}\textit{GPT-4 Usage}}
        \\
        \hline
        \multirow{8}{*}{Hint Output} & 
        Based on the given detective reasoning problem and its corresponding answer, create prompts \\&
        that concurrently aid respondents in understanding the question or the logical deduction process\\&
         without disclosing the answer outright or introducing unrelated information.\\&
         Question: ``Context + Question''\\&
         Answer: ``Answer''\\&
         You may think and reason before give the hint, please response in the following format: \\&
         ``Thinking and Reasoning Process: xxxxx\\&
         Hint: xxxxx'' \\
        \hline
        \multirow{7}{*}{Verification} & 
        Please verify the accuracy of the model's output in accordance with the provided standard answer.\\&
        If the result aligns or is similar to the standard answer, it should be deemed correct, on the contrary, \\&
        if the output from the model notably diverges from the answer, it should be considered incorrect. \\&
        Ground Truth: ``xxxx''\\&
        Model Output: ``xxx''\\&
        Please response in the following format:\\&
        ``Evaluation Result: xxxx\\&
        Evaluation Reason: xxxx''\\
        \hline
        
    \hline
    \end{tabular}
    }
    \caption{
    The prompts we used within the Self-Prompt Framework and when using the GPT-4 API.
    }
    \label{tab:prompts}
\end{table*}
\input{tables/tab_annotation_examples}
\begin{figure*}[t]
    \centering
    \resizebox{\textwidth}{!}{
    \includegraphics{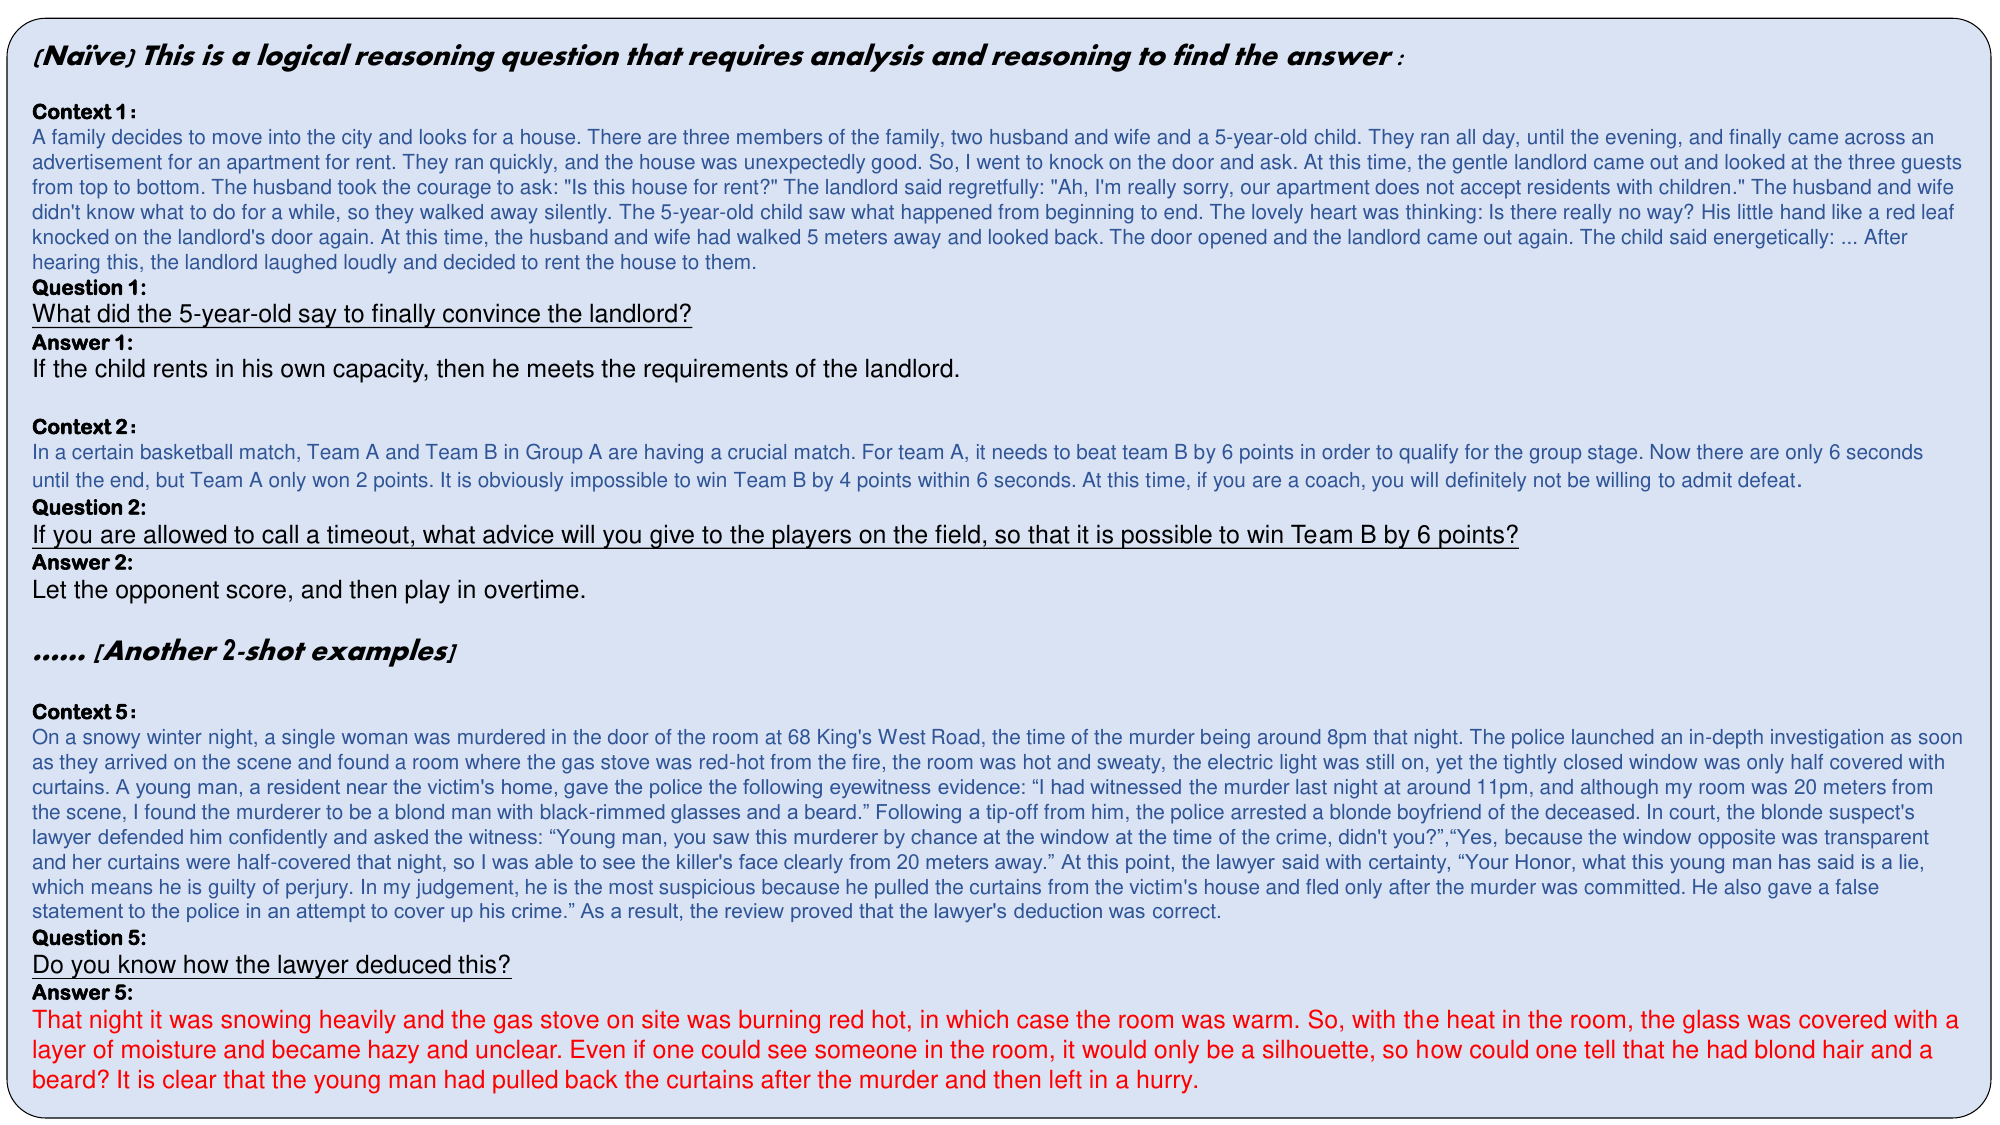}}
    \caption{Example of how we construct 5-shot demonstration in Naive setting.}
    \label{fig:naive_5shot}
\end{figure*}
\begin{figure*}[t]
    \centering
    \resizebox{\textwidth}{!}{
    \includegraphics{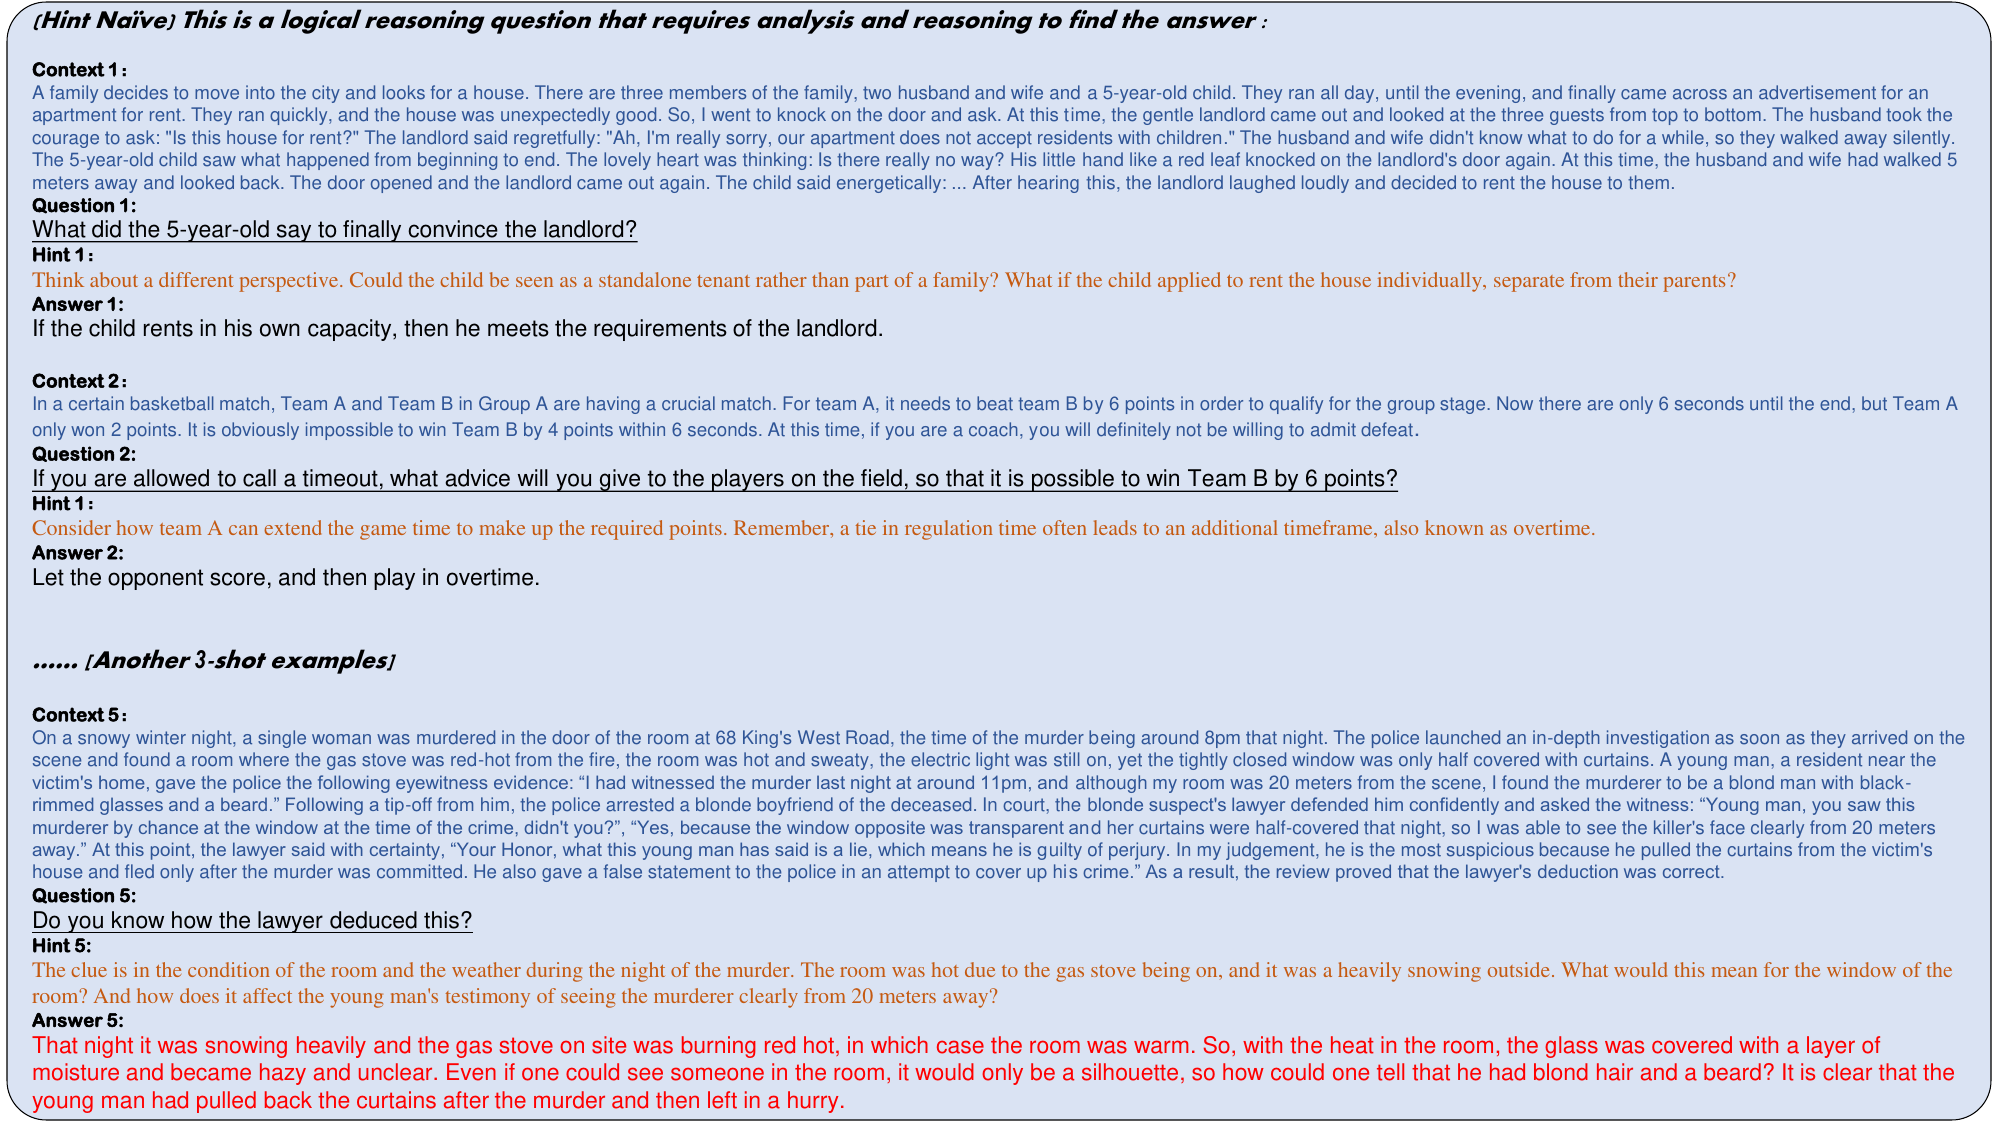}}
    \caption{Example of how we construct 5-shot demonstration in Hint-Naive setting.}
    \label{fig:hintnaive_5shot}
\end{figure*}
\begin{figure*}[t]
    \centering
    \resizebox{\textwidth}{!}{
    \includegraphics{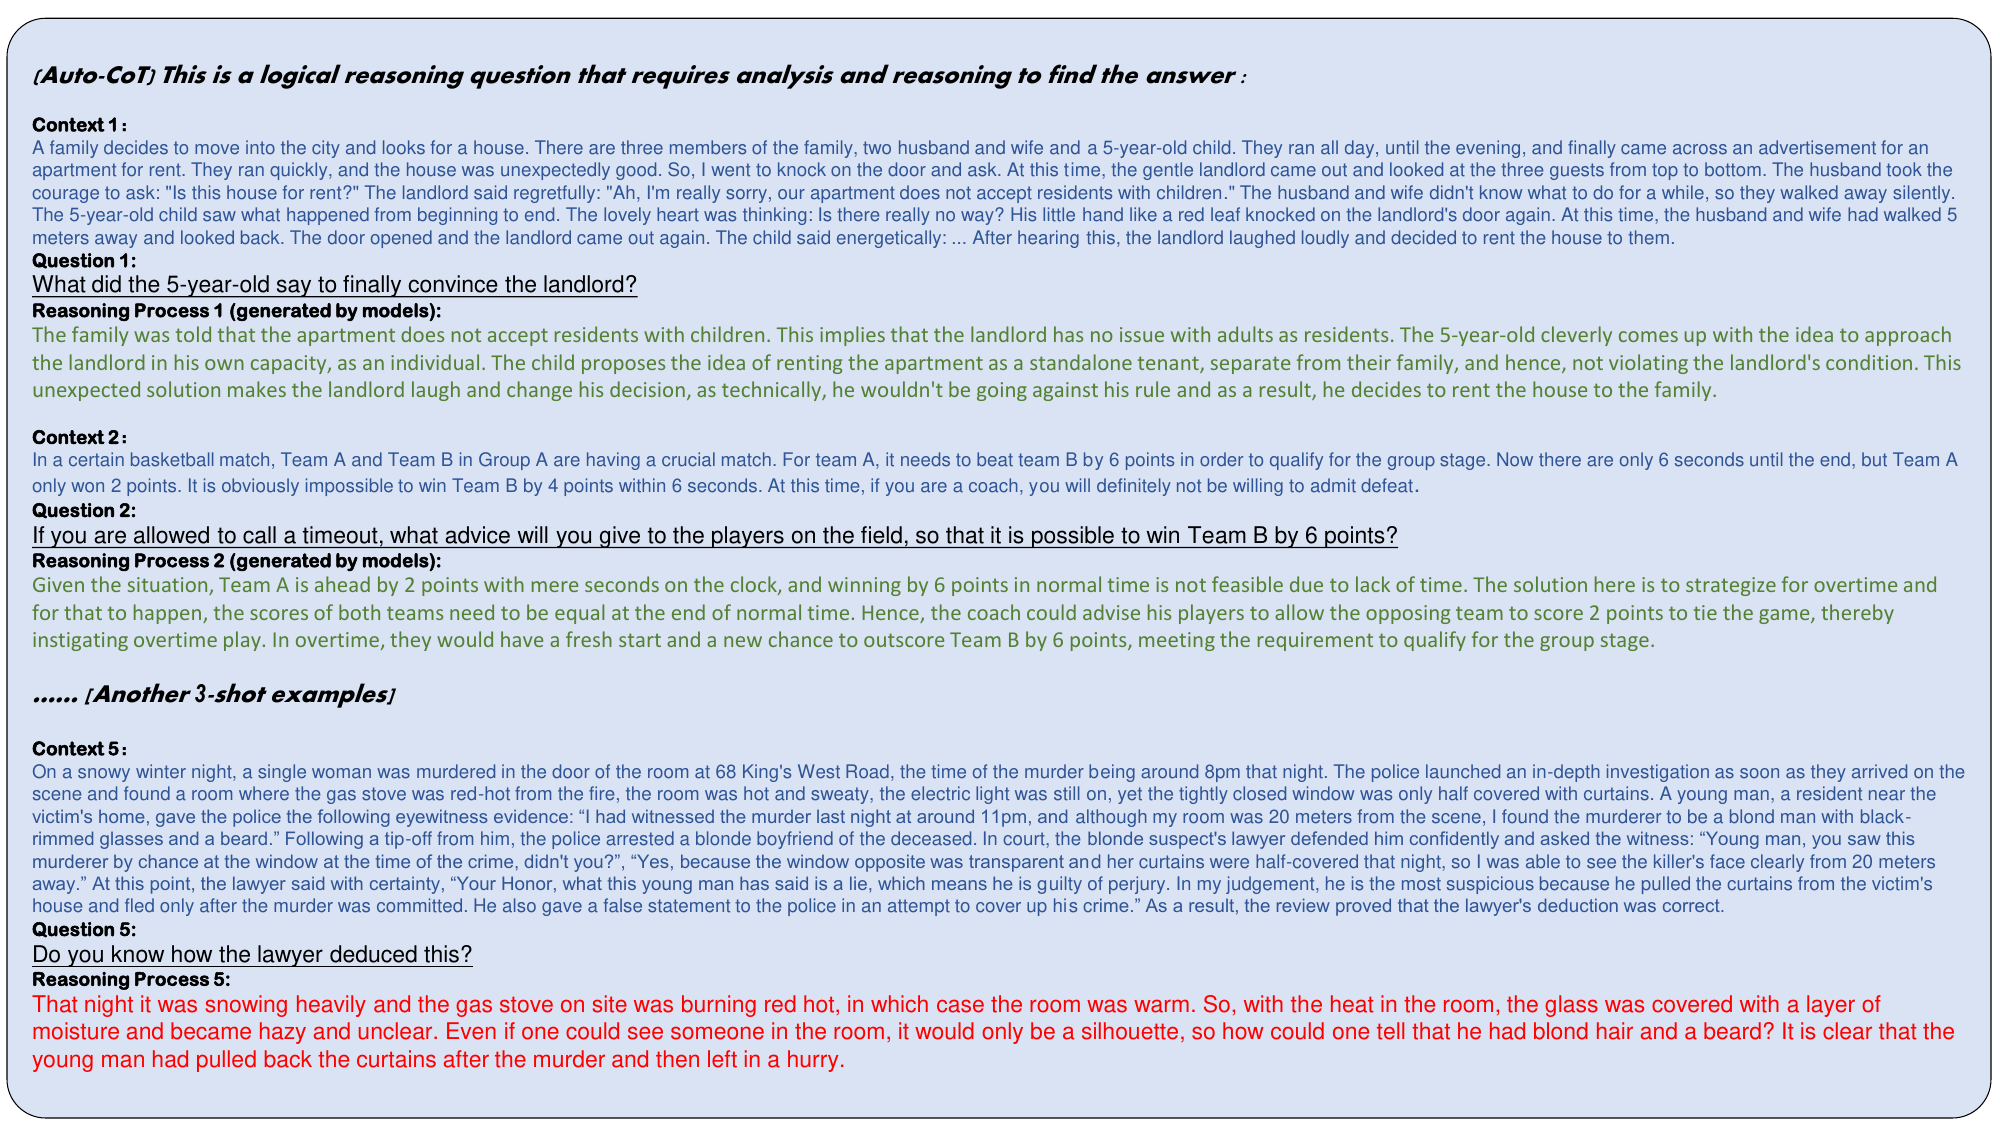}}
    \caption{Example of how we construct 5-shot demonstration in Auto-CoT setting.}
    \label{fig:autocot_5shot}
\end{figure*}
\begin{table*}[t]
\small
\centering
\resizebox{\textwidth}{!}{
\begin{tabularx}{1.6\textwidth}{|p{1.576\textwidth}|}
\hline
    \makecell[c]{\textbf{Case 1}} \\
    \hline
    \textbf{Context:} \\
    On a snowy winter night, a single woman was murdered in the door of the room at 68 King's West Road, the time of the murder being around 8pm that night. The police launched an in-depth investigation as soon as they arrived on the scene and found a room where the gas stove was red-hot from the fire, the room was hot and sweaty, the electric light was still on, yet the tightly closed window was only half covered with curtains. A young man, a resident near the victim's home, gave the police the following eyewitness evidence: 
“I had witnessed the murder last night at around 11pm, and although my room was 20 meters from the scene, I found the murderer to be a blond man with black-rimmed glasses and a beard.” 
Following a tip-off from him, the police arrested a blonde boyfriend of the deceased. In court, the blonde suspect's lawyer defended him confidently and asked the witness: 
“Young man, you saw this murderer by chance at the window at the time of the crime, didn't you?”,
“Yes, because the window opposite was transparent and her curtains were half-covered that night, so I was able to see the killer's face clearly from 20 meters away.” 
At this point, the lawyer said with certainty, 
“Your Honor, what this young man has said is a lie, which means he is guilty of perjury. In my judgement, he is the most suspicious because he pulled the curtains from the victim's house and fled only after the murder was committed. He also gave a false statement to the police in an attempt to cover up his crime.” 
As a result, the review proved that the lawyer's deduction was correct.
 \\ \\
 \textbf{Hint:}\\
 The clue is in the condition of the room and the weather during the night of the murder. The room was hot due to the gas stove being on, and it was a heavily snowing outside. What would this mean for the window of the room? And how does it affect the young man's testimony of seeing the murderer clearly from 20 meters away?
 \\
 \\
    \textbf{Question:} \\
    Do you know how the lawyer deduced this?\\
\\
\textbf{Answer:} \\
That night it was snowing heavily and the gas stove on site was burning red hot, in which case the room was warm. So, with the heat in the room, the glass was covered with a layer of moisture and became hazy and unclear. Even if one could see someone in the room, it would only be a silhouette, so how could one tell that he had blond hair and a beard? It is clear that the young man had pulled back the curtains after the murder and then left in a hurry.

\\
    \hdashline
    \textcolor{blue}{\textbf{Naive Output}}\ \xmark \\
    \textbf{Prompt:}\\
    Below is a puzzle about detective reasoning, I split the question into ``context'' and ``question'', please answer the question properly based on the context: \\
    \text{[}Context\text{]} + \text{[}Question\text{]} \\
    \textbf{Answer:} \\
    The young man claimed he saw the murder at 11pm, but the murder took place at 8pm. Furthermore, he claimed he saw it from his window 20 meters away, despite the fact that the murder victim's window was only half-open and it was a snowy night. It would be difficult to see detail like hair color, glasses, and a beard from that distance in those conditions. The lawyer concluded that the young man must have been close enough to handle the curtains, thus suspecting him of the crime.\\
    
    \hdashline
    \textcolor{blue}{\textbf{Self Chain-of-Thought}}\ \xmark \\
    \textbf{Prompt:} \\
    Below is a puzzle about detective reasoning, I split the question into ``context'' and ``question'', please answer the question properly based on the context \textit{\textbf{step by step}}: \\
    \text{[}Context\text{]} + \text{[}Question\text{]} \\
    \textbf{Answer:} \\
    Step 1: The lawyer noted inconsistencies in the young man's story. The young man claimed he witnessed the murder at 11pm, three hours after the estimated time of the murder which was around 8pm.\\
Step 2: The young man also claimed he was able to see specific details about the murderer - that he was a blond man with black-rimmed glasses and a beard - from his room 20 meters away. Given the murder took place on a snowy night, visibility would be poor.\\
Step 3: Despite the fact that the room was described as hot and sweaty, the window was only halfway open. It would be difficult to clearly observe someone from 20 meters away through a half-open window, especially during a snowy night.\\
Step 4: Based on these inconsistencies and improbabilities, the lawyer deduced that the young man was lying about what he witnessed.\\
Step 5: The lawyer then inferred that if the young man was able to see so clearly, he must not have been 20 meters away but rather close up, possibly inside the room. Therefore, the young man's close proximity and inaccurate statements made him the prime suspect in the lawyer's eyes.\\
Step 6: The lawyer argues that the young man gave a false statement to police in an attempt to cover up his own involvement in the crime. The court subsequently found these deductions to be correct. \\
    \hdashline
    \textcolor{blue}{\textbf{Manual Chain-of-Thought}}\ \cmark \\
    \textbf{Prompt:} \\
    Below is a puzzle about detective reasoning, i split the puzzle into ``context'', ``hint'' and ``question'', please answer the ``question'' properly based on ``context'' \textbf{\textit{and ``hint''}}. \\
    \text{[}Context\text{]} + \text{[}Question\text{]} + \textbf{\textit{\text{[}Hint\text{]}}}\\
    \textbf{Answer:} \\
    The lawyer deduced this from the fact that it was a snowy winter night. Due to the high temperature in the room from the gas stove, the window would have been fogged or covered with condensation on the inside because of the contrast between the warm room and the cold outside weather. This would have made it nearly impossible for the young man to clearly see the murderer's face from 20 meters away through the window, especially specific details like black-rimmed glasses and a beard. Thus, the young man's testimony was called into question, and his involvement in the crime was suspected. \\
    
    \hdashline
    \textcolor{blue}{\textbf{Plan \& Solve Chain-of-Thought}}\ \cmark \\
    \textbf{Prompt:} 
    Below is a puzzle about detective reasoning, i split the puzzle into ``context'' and ``question'', \textbf{\textit{please first understand the ``context'', extract relevant variables, and devise a plan. Then let's carry out the plan, answer the ``question'' step by step, and show the answer:}}\\
    \text{[}Context\text{]} + \text{[}Question\text{]} \\
    \textbf{Answer:} \\
    First, let's identify the relevant variables from the context:

The time of the murder: around 8pm.\\
The eyewitness saw the murder: at 11pm.\\
The distance between the eyewitness' room and the scene of the crime: 20 meters.\\
The state of the victim's room: gas stove red-hot, room hot, electric light on, closed window half covered with curtains.\\
The eyewitness' testimony: a description of the murderer; able to see the killer's face clearly from 20 meters away.\\
Based on these variables, the plan to find out how the lawyer deduced the suspicion of the witness would likely involve:\\ \\

Identifying any contradictions or inconsistencies in the statements or circumstances.\\
Evaluating the witness' testimony and its plausibility considering the conditions described.\\
Now let's carry out this plan:\\ \\

One contradiction lies in the time of the murder and the time the eyewitness claimed to have seen the murder. The murder happened around 8pm, but the witness claimed that he had witnessed the murder at 11pm.\\

Besides, the witness claimed he could see the murderer's face clearly at night from 20 meters away. Considering the physical conditions of the room described (the window was closed and only half-covered with a curtain), it seems implausible. The room was heated by a red-hot stove and the electric light was on, so the window was likely to have been steamed up, obstructing the view from outside, especially on a snowy winter night.\\

From these contradictions and implausibilities, the lawyer determined that the eyewitness was lying. His ability to describe the supposed murderer in detail, coupled with his presence at the scene (evident by his knowledge of the half-closed curtains) also raised suspicion that the eyewitness was indeed the culprit and had manipulated the scene to deceive the police. The lawyer thus accused the witness of murder, framing the blonde man, and perjury. \\
    
    \hdashline
    \textcolor{blue}{\textbf{Self-Question}}\ \cmark \\
    \textbf{Prompt:} \\
    Below is a puzzle about detective reasoning, i split the puzzle into ``context'' and ``question''. \textbf{\textit{Please first extract some key elements in the context.
    Then deduce some clue based on these elements. 
    After that, find the connection between these elements and clues to the question. 
    Finally, answer the question based on all the information.}} \\
    \text{[}Context\text{]} + \text{[}Question\text{]} \\
    \textbf{Answer:} \\
    Key Elements:\\

The crime took place around 8pm on a snowy winter night.\\
The eyewitness claimed to have witnessed the murder at 11pm.\\
The room was hot and the window was closed, but half covered with curtains.\\
The witness claimed to have seen the killer's face clearly from 20 meters away.\\ \\
Clues:\\

The difference in times that the murder took place and when the witness saw the event.\\
The conditions in the room suggest that the window was likely to have been fogged up given the heat inside.\\
The distance between the eyewitness's room and the scene makes the claim that the witness saw the murderer's face clearly suspicious.\\ \\
Connection: The lawyer focuses on the inconsistencies to doubt the reliability of the witness's testimony. The contradiction in the time of the event and the unlikelihood of the witness seeing through a likely fogged-up window from a significant distance both serve to discredit the witness.\\ \\

Answer: The lawyer deduced that the witness was lying based on the discrepancies in his testimony, namely the contradiction in the timing he reported and the implausibility of having a clear view of the murderer's face through a likely fogged-up window from a distance of 20 meters. He suspected the witness of committing the murder and fabricating the description to frame the suspect with blonde hair. The lawyer posited that the "eyewitness" was actually the real killer who had pulled the curtains, murdered the woman, and then given a false statement to divert police suspicion away from himself and towards the blonde man. \\
\hline
\end{tabularx}
}
\caption{Case study of our proposed synonym mining method and text data augmentation algorithms}
\label{tab:case1}
\end{table*}

\begin{table*}[t]
\small
\centering
\resizebox{\textwidth}{!}{
\begin{tabularx}{1.6\textwidth}{|p{1.576\textwidth}|}
\hline
\makecell[c]{\textbf{Case 2}} \\
\hline
\textbf{Context:} \\
The phone rang as the television actress, Asai Miyoko was applying her makeup at her vanity. She reached over to pick up the receiver. “Have you prepared the money yet?” her heart sank as she recognized the man’s voice on the other end. “Erm… yeah… I’m working on it…” “Well then, let's make the exchange today.” “Where?” “There’s an apartment complex near Hikari Hills Station, come to room number 508.” “What time should I come?” “Whenever it’s convenient for you?” “How about one in the afternoon?” “Okay, I’ll wait for you.” The man let out a grating laugh and ended the call. Miyoko sat still, not even remembering to put the phone back down as she stared at a small capsule she’d taken out from her vanity drawer. It contained potassium cyanide that she’d stolen when she stayed at her sister’s place who ran a pharmacy. Two years prior, she’d been coerced by a TV director into undergoing an abortion and the man now blackmailing her somehow got his hands on her medical records.
When the phone rang, the professional tennis player, Tomoya, was in the bathroom. He hurriedly rushed out to answer it. “Have you prepared the money yet?” He straightened on hearing the familiar voice, “Ah, I’m working on it…” “Well then, give me the money today.” “Where?” “There’s an apartment complex near Hikari Hills Station, come to room number 508.” “When?” “Two in the afternoon. I’ll be waiting for you.” The man laughed and hung up. Tomoya thought for a long while before pulling out a small medicine bottle from his drawer. It contained potassium cyanide that he’d stolen from his wife’s electroplating factory’s poison cabinet a day ago.
The phone rang as the innocent pop idol, Kato Mayumi, was eating breakfast alone in her kitchen. “Did you prepare the money I asked for?” Her body shivered as she recognized the man’s voice over the phone. “Erm… well…” “Give me the money today.” “Where?” “There’s an apartment complex near Hikari Hills Station, come to room number 508.” She replied, “Erm… I had plans to go driving around for fun today…” He responded, “Do you think your little trip is more important than our transaction here? Anyway, you can come anytime between one and three, I’ll be waiting.” The man menacingly ended the call.
 \\ \\
 \textbf{Hint:}\\
 Observe the temperature inside the room, the status of the windows, you will find contradictory clues. Look for phenomena that only occur during a power outage.
 Potassium cyanide, if it is in contact with the air for a long time, will turn into potassium carbonate and lose its toxicity. One suspect's potassium cyanide has been stored for two years, so consider what changes might have occurred.
 Take note of the different references by suspects to the air conditioning, elevator, and power outage. These could reveal key aspects of the suspect’s actions.
 Read carefully through each person's actions. You'll find one person's actions differ from the others, which might be a key clue to the culprit.
 In the afternoon, from half-past one to half-past two, one suspect arrived at the apartment during the power outage. What method did they use to get in?
 \\
 \\
\textbf{Question:} \\
Who among the three used the potassium cyanide to murder the blackmailer and why?\\
\\
\textbf{Answer:} \\
The murder took place during a power outage. Due to the outage, the air conditioner stopped working and the room became hot, causing the victim to open the window themselves. If the victim was still alive when the power was restored and the air conditioner started working again, they would have closed the window. Only Tomoya and Mayumi visited the scene during the power outage. However, who killed the victim with their potassium cyanide? If potassium cyanide is not stored in an airtight container and is exposed to air for a long period, it will turn into potassium carbonate and lose its toxicity. The potassium cyanide Mayumi had was wrapped in paper for two years, and thus, had already lost its potency. \textbf{\textit{Therefore, the murderer is Tomoya.}}

\\
\hdashline
\textcolor{blue}{\textbf{Naive Output}}\ \xmark \\
\textbf{Prompt:}\\
Below is a puzzle about detective reasoning, I split the question into ``context'' and ``question'', please answer the question properly based on the context: \\
\text{[}Context\text{]} + \text{[}Question\text{]} \\
\textbf{Answer:} \\
\textbf{\textit{Kato Mayumi.}} Although all three suspects have the motive and means to kill the blackmailer, the timing of the power outage in the apartment suggests only Mayumi had the chance to do so. The elevator in the blackmailer's home could not operate after the power went off, so only the person who arrived before the power outage (Mayumi) could have seen him before he was killed. The other two people, one couldn't take the elevator due to the blackout and had to climb the stairs, while the other left when the elevator was stuck on the first floor, so neither of them had the chance to see the blackmailer before the power outage.\\

\hdashline
\textcolor{blue}{\textbf{Self Chain-of-Thought}}\ \xmark \\
\textbf{Prompt:} \\
Below is a puzzle about detective reasoning, I split the question into ``context'' and ``question'', please answer the question properly based on the context \textit{\textbf{step by step}}: \\
\text{[}Context\text{]} + \text{[}Question\text{]} \\
\textbf{Answer:} \\
Firstly, if Miyoko's elevator descended to the first floor when the power went off, it means that the other two have already been to the scene, otherwise Miyoko should have been trapped in the dark elevator. So, Miyoko is the last one to leave the scene.\\

Secondly, Tomoya went up the stairs, and he mentioned that he encountered two housewives. If he was the criminal, he wouldn't have allowed the two housewives to see him exit the stairwell, as that would serve as incriminating evidence.\\

Thirdly, Mayumi mentioned that onlookers were staring at her. If she was seen leaving the apartment, wouldn't that be very dangerous?\\

From these clues, it is most likely that \textbf{\textit{Miyoko killed the blackmailer}}. Because she was the last one to leave the scene, and due to the power outage, the elevator stopped operating, she wouldn't encounter anyone else, therefore there was no risk of being seen leaving the apartment.\\
\hdashline
\textcolor{blue}{\textbf{Manual Chain-of-Thought}}\ \cmark \\
\textbf{Prompt:} \\
Below is a puzzle about detective reasoning, i split the puzzle into ``context'', ``hint'' and ``question'', please answer the ``question'' properly based on ``context'' \textbf{\textit{and ``hint''}}. \\
\text{[}Context\text{]} + \text{[}Question\text{]} + \textbf{\textit{\text{[}Hint\text{]}}}\\
\textbf{Answer:} \\
\textbf{The answer is Tomoya.} He is the only one who arrived at the apartment during the power outage, and because the elevator was out of service, he had to take the stairs. He also mentioned encountering two housewives on the stairs, which indicates that the elevator was already out of order at that time. However, he did not mention that the air conditioning in the room was on, which conflicts with the statements of the other two suspects. Only those who took the elevator upstairs would know that the room's air conditioning would also stop working after the power outage. This suggests that he had already arrived at the apartment before the power outage, therefore the victim's time of death was before the power cut, which is when he arrived. Moreover, the potassium cyanide was just obtained by him last night, so it couldn't undergo a chemical change to become non-toxic. Therefore, the murderer who poisoned the victim is Tomoya. \\

\hdashline
\textcolor{blue}{\textbf{Plan \& Solve Chain-of-Thought}}\ \xmark \\
\textbf{Prompt:} 
Below is a puzzle about detective reasoning, i split the puzzle into ``context'' and ``question'', \textbf{\textit{please first understand the ``context'', extract relevant variables, and devise a plan. Then let's carry out the plan, answer the ``question'' step by step, and show the answer:}}\\
\text{[}Context\text{]} + \text{[}Question\text{]} \\
\textbf{Answer:} \\
Context:\\

We have three characters who are being blackmailed: The television actress, Asai Miyoko; the professional tennis player, Tomoya; and the pop idol, Kato Mayumi. They were all asked to go to an apartment complex near Hikari Hills Station, room number 508. Miyoko's meeting is at one in the afternoon, Tomoya's at two in the afternoon, and Mayumi can come anytime between one and three in the afternoon. Both Miyoko and Tomoya have stolen potassium cyanide, which is extremely poisonous.\\ \\ 

Plan: \\

Understand the chronology of events, like what times are specified for each person to meet with the blackmailer.
Analyze the opportunities each person would have had to use the cyanide.
Determine the individual motive for each person.\\ \\ 
Execution:\\

Miyoko is supposed to meet the blackmailer at 1 PM. This gives her the first opportunity to meet the blackmailer and potentially poison him before the others arrive. Tomoya comes next at 2 PM. Mayumi can come anytime between 1 PM and 3 PM.
Both Miyoko and Tomoya have potassium cyanide, so both could potentially poison the blackmailer if they have the opportunity to do so.
Everyone has a motive to kill the blackmailer as he is threatening their lives, and they all have been violated by him in different ways.\\
Based on this analysis, \textbf{\textit{the most likely person to have used the potassium cyanide to murder the blackmailer would be Miyoko}}, primarily because she is the first one scheduled to meet with him, providing her the opportunity to poison him before the others arrive.
However, without evidence that the blackmailer is indeed dead, and without knowing whether the blackmailer met Miyoko first or violated the arranged schedule, we can't say with 100\% certainty who would or wouldn't have had the opportunity to murder the blackmailer. \\
    
\hdashline
\textcolor{blue}{\textbf{Self-Question}}\ \cmark \\
\textbf{Prompt:} \\
Below is a puzzle about detective reasoning, i split the puzzle into ``context'' and ``question''. \textbf{\textit{Please first extract some key elements in the context.
Then deduce some clue based on these elements. 
After that, find the connection between these elements and clues to the question. 
Finally, answer the question based on all the information.}} \\
\text{[}Context\text{]} + \text{[}Question\text{]} \\
\textbf{Answer:} \\
Key elements:\\

Asai Miyoko, the television actress, is asked to come to room number 508 at an apartment complex near Hikari Hills Station at one in the afternoon. She has potassium cyanide.\\
Tomoya, the professional tennis player, is asked to come to the same room at two in the afternoon. He also has potassium cyanide.
Kato Mayumi, the pop idol, is asked to come to the same room anytime between one and three in the afternoon.\\\\
Clues:\\

All three are being blackmailed and have access to potassium cyanide.\\
The blackmailer has different meeting times with each person.\\
Connection: The meeting times are crucial. The blackmailer is meeting Miyoko at one, Tomoya at two, and Mayumi anytime between one and three.\\\\

Answer:\\
\textbf{\textit{Tomoya, the professional tennis player, is the most likely to have used the potassium cyanide to murder the blackmailer.}} This is because he was scheduled to meet the blackmailer after Miyoko, meaning the blackmailer would still be alive when she arrived. Mayumi could have potentially been the murderer, but since her time slot overlaps with both Miyoko and Tomoya, it's less certain. Tomoya, however, was scheduled to meet the blackmailer alone, giving him the perfect opportunity to commit the crime.\\
\hline
\end{tabularx}
}
\caption{Case study of our proposed synonym mining method and text data augmentation algorithms}
\label{tab:case2}
\end{table*}

% \subsection{Prompts Used in Experiments}
% \label{appendix_prompts}
% The detail prompts we used in all our experiments are listed in Tab.~\ref{tab:prompts}

\subsection{Limitation}

\textbf{Limitations of the Detective Reasoning Puzzle Benchmark}

The Detective Reasoning Puzzle Benchmark is designed for evaluating the informal reasoning ability of both humans and machine learning models.
Nonetheless, the benchmark only partially reflects the informal reasoning capabilities of humans and machine learning models, as it only consists of textual tasks.
Moreover, compared to the information faced in real-life, the information provided in detective reasoning puzzles is significantly more condensed.
As the name of our benchmark suggests, Detective Reasoning Puzzles Benchmark emphasizes on evaluating informal reasoning predominantly from a detective reasoning perspective, though even textual tasks should embody a variety of different types of tasks to adequately evaluate informal reasoning.

\textbf{Limitations of the Self-Question Prompt}

In our experiments, the Self-Question Prompt proves effective to improve model's performance on Detective Reasoning Puzzles Benchmark by restoring the process of human-like informal reasoning.
However, this method is only applicable to tasks that require extraction and inferencing of key information from a wealth of data.
It work poorly when the available information is scant and need to add information based on common sense or experience.
Besides, to equip machine learning models with human-like informal reasoning abilities, improvement should be made in model parameters and structure, Self-Question is merely a palliative method.

% \textbf{Limitation of Detective Reasoning Puzzle Benchmark}
% Detective Reasoning Puzzle Benchmark is proposed for evaluating the informal reasoning ability of humans and Machine Learning Models.
% 然而，这份数据集只能部分体现出人类和机器的informal reasoning的能力，因为这份数据集只聚焦在文本任务，而且相较于真实生活中所需要面对的信息量，detective puzzles所包含的信息量已经相当少了。
% 另外，如这份数据集的名字所示，这份数据集主要聚焦从侦探推理的角度评估informal reasoning，而即便是只用文字，informal reasoning都应该体现在更多不同类型的任务中。

% \textbf{Limitation of Self-Question Prompt}
% Self-Question Prompt被我们的实验证实因为能够还原人类进行informal reasoning的过程，从而能够有效提升模型在informal reasoning任务上的效果。
% 但这种方法只适用于已有大量的信息，从中提取关键信息并进行推理的任务。
% 当信息量过少，需要自动补全所有信息时，Self-Question方法便会大打折扣。
% 此外，真正需要让模型具备类人的Informal reasoning能力，还是需要从模型参数以及结构上着手进行改进，self-question只是一种缓解方案。

\subsection{Experimental Deployment of Prompts} 
The meticulous selection and usage of prompts play a pivotal role in the experimental design.
In our endeavor to maintain transparency and facilitate a comprehensive understanding of the procedures, we have elucidated these prompts in accordance with their application across the different experiments.
The catalog of prompts, annexed in Tab.~\ref{tab:prompts}, provides a detailed view of the specific prompts utilized in every individual experiment.

\subsection{Detail about Manual Annotation}
\label{appendix_annotators}
\subsubsection{Details about Annotators}
The annotators for this research are the authors of this paper themselves, who are experts in the field of Computer Science and Cognitive Psychology.
% Respecting the requirement for anonymity, specific details regarding the number and education degrees of the annotators are not elaborated here.
% It can be shared that the annotators are experts in the field of Computer Science and Cognitive Psychology.
The entire annotation process was under the stringent supervision and scrutiny of the first author of this paper.
\subsubsection{Annotation Tasks and Goals}
The purpose of the manual annotation tasks was twofold.
The first goal was to obtain comprehensive annotated datasets that encapsulate the essential features of the target text, which could be further leveraged for tasks such as training, testing, and model evaluation.
The second goal was to provide a detailed, rigorous, and systematic assessment of the annotated data quality to assess its fit and reliability for the subsequent analysis.
All the detailed annotation tasks and targets are listed in Tab.~\ref{tab:annotation_request}.
\subsubsection{Case of Annotation}
In our efforts to delineate the complex annotation process and ensure the replicable rigor of experiments, this section provides an in-depth display of the manual annotation cases.
The aim is to elucidate the categorical distinctions and precise definitions adopted in the annotations, thereby facilitating fellow researchers in ascertaining the veracity of the annotated data.
Representative cases from the annotation process have been cataloged in Tab.~\ref{tab:appendix_annotation_example} for comprehensive reference and understanding.

\subsection{Demonstration Construction}
\label{appendix_demonstration}
This subsection lays bare the intricate procedure undertaken to construct a 5-shot demonstration for each of the proposed baselines.
It is imperative to note that the 5-shot demonstration was utilized within the purview of \texttt{Naive}, \texttt{Auto-CoT}, and \texttt{Hint-Naive} settings as posited in Tab.~\ref{experiments}. 
Fig.~\ref{fig:naive_5shot}, Fig.~\ref{fig:hintnaive_5shot} and Fig.~\ref{fig:autocot_5shot} elucidate how we add the questions in the training set together, revealing the detailed construction that underpin them.

\subsection{Case Study}
In pursuit of shedding light on the practical aspects and implications of the proposed models, this section provides cases gleaned from the gamut of experiments conducted. Two such selected cases, emblematic of the diversity in application and the robust adaptability of the models, have been tabled in Tab.~\ref{tab:case1} and Tab.~\ref{tab:case2}.
